# Supplementary material for: Im4D: High-Fidelity and Real-Time Novel View Synthesis for Dynamic Scenes
Source: arXiv:2310.08585 source file (2023-10-12)
Supplement: Supplementary file 1 [file supp_sport1.tex]

\begin{table}
    \tabcolsep=0.1 cm
    \begin{center}
    \caption{\textbf{Quantitative ablation of view synthesis results on NHR and DNA-Rendering datasets.} Tt represents the training time, and its corresponding unit is hours. The detailed descriptions can be found in Sec. \ref{sec:ablation}.}
    \label{tab:ab_zju_nhr}
    \resizebox{\columnwidth}{!}{
    \begin{tabular}{l|ccc|ccc}
    \Xhline{3\arrayrulewidth}
     &  \multicolumn{3}{c|}{NHR} & \multicolumn{3}{c}{DNA-Rendering} \\
    % \hline
    %  & PSNR $\uparrow$ & SSIM $\uparrow$ & LPIPS $\downarrow$ & PSNR $\uparrow$ & SSIM $\uparrow$ & LPIPS $\downarrow$ & FPS  $\uparrow$ \\
      & PSNR $\uparrow$  & LPIPS $\downarrow$  & Tt $\downarrow$ & PSNR $\uparrow$  & LPIPS $\downarrow$  & Tt $\downarrow$ \\
    \hline
    1) Complete model & 34.87 & 0.043 & 2.29 & 29.82 & 0.045 & 3.33  \\
    2) w/o \textit{image-based} appearance &  31.79 & 0.107 & 1.81 & 26.07 & 0.102 & 2.54  \\
    3) w/o \textit{global} geometry     &  24.71 & 0.152 & 2.81 & 27.44 & 0.100 & 4.04  \\
    % 4) IBRNet     &  34.65 & 0.068 & 2.00 & 32.40 & 0.962  \\
    \hline
    4) $\numJointTraining = 0$, \quad\, $\numFinetuneTraining = \infty$ & 30.44 & 0.051 & 2.21 &  28.25 & 0.047 & 3.23 \\
    5) $\numJointTraining = 0$, \quad\, $\numFinetuneTraining = 20$  & 34.30 & 0.044 & 2.25 & 29.63 & 0.047 & 3.29 \\
    6) $\numJointTraining = 5000$, $\numFinetuneTraining = \infty$ & 34.29 & 0.043 & 2.26 & 29.27 & 0.045 & 3.27 \\
    7) $\numJointTraining = \infty$, \quad $\numFinetuneTraining = \textbackslash$ &34.89 & 0.042 & 3.19 & 29.83 & 0.045 & 4.55 \\ \hline
    8) w/o pre-trained model & 35.11& 0.042 & 2.29 & 29.58 & 0.047 & 3.33 \\  \hline
    9) \textit{inferring} ability & 34.82& 0.045 & 2.26 & 29.00 & 0.050 & 3.27 \\ 
    \Xhline{3\arrayrulewidth}
    \end{tabular}
    }
    \end{center}
\end{table}
